# Supplementary material for: Deduction under Perturbed Evidence: Probing Student Simulation Capabilities of Large Language Models
Source: arXiv:2305.14507 source file (2023-05-23)
Supplement: Supplementary file 1 [file appendix.tex]

hello
